# Supplementary material for: Transformers in Time Series: A Survey
Source: arXiv:2202.07125 source file (2023-05-11)
Supplement: Supplementary file 1 [file 8_Appendix.tex]

\section{Appendix: xxx}\label{subsec:data-aug}
